# Supplementary material for: Coupling between Inclusions and Membranes at the Nanoscale
Source: arXiv:1803.10089 source file (2018-03-27)
Supplement: Supplementary file 1 [file Bories_SM_rev.pdf]

# Supplemental Material: "Coupling between inclusions and membranes at the nanoscale"

Florent Bories,[1] Doru Constantin,[2,*] Paolo Galatola,[1,†] and Jean-Baptiste Fournier[1,‡]

[1]*Laboratoire "Matière et Systèmes Complexes" (MSC), UMR 7057 CNRS, Université Paris 7 Diderot, 75205 Paris Cedex 13, France*

[2]*Laboratoire de Physique des Solides, CNRS, Univ. Paris-Sud, Université Paris-Saclay, 91405 Orsay Cedex, France.*

## I. GENERAL FORM OF THE ELASTIC FREE-ENERGY DENSITY

We assume that the deformation free energy of a membrane undergoing symmetric thickness variations $u(\boldsymbol{r})$ on both sides of a flat midsurface can be expressed as

$$F = \int d^2r\, f(u, u_i, u_{ij}), \tag{1}$$

where $u_i = \partial_i u$ and $u_{ij} = \partial_i \partial_j u$ are partial derivatives with respect to a coordinate system in the plane of the membrane midsurface, on which the integral is performed. Including in $f$ all the scalar terms up to quadratic order yields

$$f = Au + A_i u_i + A_{ij} u_{ij} + Bu^2 + C_i u u_i + D_{ij} u u_{ij} + E_{ij} u_i u_j + F_{ijk} u_i u_{jk} + G_{ijk\ell} u_{ij} u_{k\ell}, \tag{2}$$

where the Einstein summation over repeated dummy indices is implied and all the coefficients are scalars or tensors of order 1 to 4. Because the membrane is isotropic all the tensors of odd order must vanish, i.e., $A_i = C_i = F_{ijk} = 0$. The other tensors can be written in terms of the identity tensor: $A_{ij} = a\delta_{ij}$, $D_{ij} = d\delta_{ij}$, $E_{ij} = e\delta_{ij}$ and $G_{ijk\ell} = g_1\delta_{ij}\delta_{k\ell} + g_2\delta_{ik}\delta_{j\ell} + g_3\delta_{i\ell}\delta_{jk}$. Because $u_{ij}$ is symmetric, $g_2$ and $g_3$ yield the same contribution, and thus we can set $g_3 = 0$ without loss of generality. We can also set $A = 0$ if we assume that $u$ is the thickness variation relative to the *equilibrium thickness*. Hence we arrive at

$$f = au_{ii} + Bu^2 + duu_{ii} + eu_i u_i + g_1 u_{ii} u_{jj} + g_2 u_{ij} u_{ij}. \tag{3}$$

Using the identities $uu_{ii} = \partial_i(uu_i) - u_i u_i$ and $u_{ij}u_{ij} = u_{ii}u_{jj} - 2\det(u_{ij})$, we can rewrite $f$ as

$$f = Bu^2 + (e-d)(\nabla u)^2 + (g_1+g_2)(\nabla^2 u)^2 + a\nabla^2 u + d\nabla\cdot(u\nabla u) - 2g_2 \det(u_{ij}). \tag{4}$$

Upon normalizing and changing the name of the coefficients, this form is equivalent to Eq. (1) in the main text.

The lipid tilt degrees of freedom are not included in our elastic theory. This is not a limitation, however, since according to equilibrium statistical mechanics they can be coarse-grained out, being free to adjust to equilibrium. Hence our elastic free energy, function of the membrane thickness only, can be considered as having been already optimized with respect to the underlying tilt degrees of freedom, for any given thickness profile.

### A. Surface tension

In our experiments and those that we analyze, the lamellar phases are not subject to any explicit external tension and are therefore expected to have only small residual tensions $\sigma$. Moreover, $\sigma$ influences the interaction between inclusions only at distances larger than $\sqrt{\kappa_0/\sigma}$. Now, the range of our interaction potentials is of the order of 10 Ångstroms. Therefore, $\sigma$ can be safely neglected since to influence the interaction at this scale it should be of the order of 0.05 N/m, which is roughly 5 times the lysis tension of the membrane. See Ref. 1 for a more complete discussion.

### B. Tilt of the inclusion

Both the channel and the bilayer are symmetric with respect to the inversion $z \to -z$, forbidding a net bending of the membrane. This symmetry can be spontaneously broken, but the gramicidin channel is a rigid and wide object, with low mismatch (only 2.1 Å) with respect to DLPC. Recent numerical simulations [2, 3] report a modest tilt angle, of the order of 15°. It is therefore reasonable to neglect the bending deformation of the membrane.

### C. Intermembrane interaction

Throughout the paper, we have assumed that the gramicidin channels only interact within the same membrane, and not between adjacent membranes. This assumption is justified by literature results [4] showing that uncharged channels (formed by alamethicin) at full hydration do not exhibit intermembrane correlations. Gramicidin is uncharged and our samples are fully hy-

* doru.constantin@u-psud.fr
† paolo.galatola@univ-paris-diderot.fr.
‡ jean-baptiste.fournier@univ-paris-diderot.fr.

drated (in excess water), so we do not expect any intermembrane interaction.

## II. FITTING DETAILS

The statistical error in the $S(q)$ data is very low, as can be seen from the scatter in the data points of Fig. 2, and would result in small error bars and a huge $\chi^2$ function. The major sources of error are systematic, *e.g.* due to background subtraction and division by the form factor or to discrepancies between the model and the data, but it is impossible to estimate their variation with $q$. Following Ref. 10, we use a conservative uncertainty of 0.1 for all data points, yielding a $\chi^2$ of the order of 1 per point. Of course, any other constant value would yield the same results for the fit parameters.

## III. COMPARISON WITH THE ANALYSIS IN REF. 5

The structure factors $S(q)$ had already been analyzed in Ref. 5 ([10] in the main text) using a different model. In this section, we compare the interaction potentials obtained via the two approaches.

The phenomenological analysis in Ref. 5 relies on an ad-hoc assumption, namely that the interaction potential decreases with the concentration of inclusions, and the $V(r)$ potential presented corresponds to low concentration. The more rigorous study presented here does not require this assumption. Thus, the two potentials do not have quite the same significance. Furthermore, because most experimental spectra are compared to a weaker potential, the low concentration potential of Ref. 5 is severely overestimated, as can be seen in Figure 1. Finally, in Ref. 5 the structure factors are obtained from $V(r)$ using the Percus-Yevick closure, which is not well adapted in this context (as we have realized after comparison with the Monte Carlo results).

Thus, the new analysis improves on the previous one both quantitatively (less assumptions, a more rigorous implementation method and a different shape of the potential) and qualitatively (relating the potential to the underlying elastic theory).

## IV. MATERIAL CONSTANTS FOR THE BILAYER ELASTICITY

*DMPC.* We set $d_0 = 25.4\,\text{Å}$, $\kappa_0 = 0.63 \times 10^{-19}\,\text{J}$, $\bar{\kappa} = -0.8\kappa_0$ and all the other parameters equal to those of DLPC [6].

*DPPC.* We set $d_0 = 28.5\,\text{Å}$, $\kappa_0 = 0.8 \times 10^{-19}\,\text{J}$, $\bar{\kappa} = -0.8\kappa_0$ and all the other parameters equal to those of DLPC [6].

*DSPC.* We set $d_0 = 32.5\,\text{Å}$, $\kappa_0 = 1.04 \times 10^{-19}\,\text{J}$, $\bar{\kappa} = -0.8\kappa_0$ and all the other parameters equal to those of DLPC [6].

*DOPC.* We use the following literature data [5–7] for the known material constants of DOPC: $K_a = 0.265\,\text{N}\,\text{m}^{-1}$, $d_0 = 27\,\text{Å}$, $\kappa_0 = 0.85 \times 10^{-19}\,\text{J}$, $\bar{\kappa} = -0.8\kappa_0$, $c_0 = -0.0132\,\text{Å}^{-1}$, $c_0' \simeq 0\,\text{Å}$.

## V. MULTIPOLE EXPANSION

In our model, each gramicidin inclusion imposes, as per the hydrophobic matching principle, a fixed excess thickness

$$u(r_0, \phi) = u_0 \tag{5}$$

along its boundary $r = r_0$, where $(r, \phi)$ are polar coordinates centered on the inclusion. Since the elastic energy includes second-order derivatives, the equilibrium thickness profile depends on the radial derivative of $u$ along the boundary. We therefore assume that the inclusions set a preferred angle via a quadratic boundary potential per unit length. The latter can be written in two equivalent forms:

$$\begin{aligned} g &= \frac{1}{2} w \left(\partial_r u|_{r_0} - s\right)^2 \\ &= -\tau\, \partial_r u|_{r_0} + \frac{1}{2} w \left(\partial_r u|_{r_0}\right)^2 + \text{cst.} \end{aligned} \tag{6}$$

where $w$ is an anchoring strength, $s$ the tangent of the preferred angle, and $\tau \equiv ws$ is the torque exerted by the inclusion when the boundary angle vanishes. According to the magnitude of $w$, we can distinguish three cases: (i) weak anchoring, where one can set $w = 0$ without changing substantially the membrane profile $u$, (ii) strong anchoring, which amount to letting $w \to \infty$ in (6), and (iii) intermediate strength, where $\partial_r u|_{r_0}$ is generally different from $s$, but the effect of the anchoring on the profile is considerable. Only cases (i) and (ii) were used in the literature [1, 7, 8], with various values of $s$.

The equilibrium profile is obtained by minimizing the total free energy, yielding the equations:

$$\left(\nabla^2 - \lambda_+^2\right)\left(\nabla^2 - \lambda_-^2\right) u = 0, \tag{7}$$

$$a_1 + a_2 u + k_2 \nabla^2 u + \bar{k} \frac{\partial_r u}{r} - w\left(\partial_r u - s\right)\Big|_{r_0} = 0, \tag{8}$$

where $\lambda_\pm^2 = (k_1 \pm \sqrt{k_1^2 - 4k_2})/(2k_2)$, supplemented with Eq. (5). The stability of the membrane requires $k_2 > 0$ and $k_1 > -2\sqrt{k_2}$ [9]. Note that for $k_1 > 2\sqrt{k_2}$ the roots $\lambda_\pm$ are real; they are complex otherwise.

For two inclusions, by virtue of linearity and symmetry, the most general solution of Eq. (7) that vanishes at

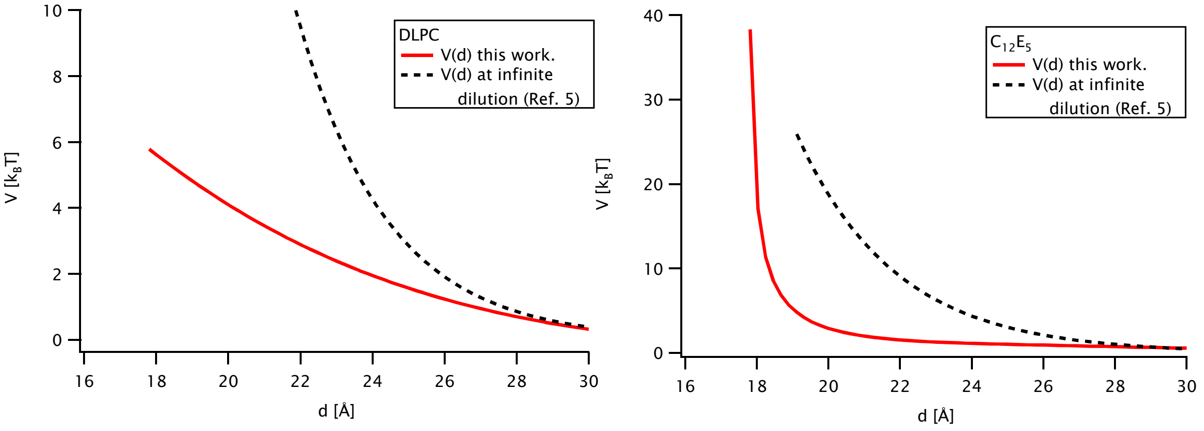


FIG. 1. Interaction energy $V$ between two gramicidin channels as a function of their center-to-center distance $d$ in DLPC (left) and $C_{12}E_5$ (right) bilayers. Solid red line: this work. Dashed black line: Interaction energy at infinite dilution in Ref. 5.

infinity can be written as the multipolar expansion

$$u = v(r_1, \phi_1) + v(r_2, \phi_2), \tag{9}$$

$$v(r, \phi) = \sum_{n=0}^{\infty} [A_n K_n(\lambda_+ r) + B_n K_n(\lambda_- r)] \cos(n\phi), \tag{10}$$

where $r_{1,2}$ and $\phi_{1,2}$ are polar coordinates centered on the inclusions (see Fig. 1 in the main text), the $K_n$ are modified Bessel functions of the second kind and order $n$, and $\lambda_\pm$ have positive real parts. The boundary conditions (5) and (8) determine all the unknown multipolar coefficients $A_n$ and $B_n$ in Eq. (10) in the form of an (infinite) linear system. We solve the latter numerically by neglecting all the multipoles above a certain rank and checking for convergence as the rank is increased.

## VI. SIMULATED MEMBRANE PROFILES

1. Chiu et al. [10] studied one channel surrounded by 96 DMPC molecules in excess water and found that the membrane thickness was decreasing away from the channel in its immediate vicinity, in contrast with the increase expected from the difference in hydrophobic length.

2. Yoo and Cui [11] performed all-atom simulations of one channel surrounded by 72 DMPC or DSPC molecules. In both cases, the membrane profile exhibits a steep decrease away from contact, followed by a slower increase to its equilibrium value away from the inclusion (see their Figure 4A). This behavior is lost in coarse-grained systems, where the increase is monotonic (see their Figure 4B).

3. More recently, Beaven et al. [12] performed all-atom simulations of one channel surrounded by 180 lipid molecules of different types. In pure di-eicosenoyl-phosphocholine bilayers, the hydrophobic thickness profile decreases steeply away from the boundary before increasing up to the equilibrium value (their Figure 7).

## VII. FORMATION RATE OF THE CHANNELS UNDER TENSION

Let us calculate the elastic energy stored in the membrane for a single channel. The solution of Eq. (4) of the main text, with revolution symmetry in polar coordinates, is given by

$$u(r) = A_+ K_0(\lambda_+ r) + A_- K_0(\lambda_- r). \tag{11}$$

Satisfying the boundary conditions Eqs. (2) and (5) of the main text yields

$$A_\pm = \frac{(wr_0 - \bar{k}) K_1^\mp \lambda_\mp u_0}{\pm D} + \frac{K_0^\mp r_0 (a_1 + a_2 u_0 + sw + k_2 u_0 \lambda_\mp^2)}{\pm D}, \tag{12}$$

where

$$K_0^\pm = K_0(\lambda_\pm r_0), \tag{13}$$

$$K_1^\pm = K_1(\lambda_\pm r_0), \tag{14}$$

$$D = (wr_0 - \bar{k})(K_0^- K_1^+ \lambda_+ + K_0^+ K_1^- \lambda_-) + K_0^+ K_0^- k_2 r_0 (\lambda_-^2 - \lambda_+^2). \tag{15}$$

Since $u(r)$ is solution to the Euler-Lagrange equation, the total elastic energy

$$F = \int_{r>r_0} f\, d^2r + 2\pi r_0 g\,, \tag{16}$$

where $f$ and $g$ are given by Eqs. (1) and (3) of the main text, respectively, can be transformed by integration by

parts into

$$\frac{F}{\pi r_0} = \Bigg[ - k_1 u_0 \frac{\partial u}{\partial r} + k_2 u_0 \frac{\partial \nabla^2 u}{\partial r} - k_2 \nabla^2 u \frac{\partial u}{\partial r} - 2(a_1 + a_2 u_0) \frac{\partial u}{\partial r} - \frac{\bar{k}}{r} \left( \frac{\partial u}{\partial r} \right)^2 + w \left( \frac{\partial u}{\partial r} - s \right)^2 \Bigg]_{r_0} . \quad (17)$$

With $u(r)$ given by Eqs. (11) and (12), we obtain $F$ as a function of the parameters of the model.

The dimensionless hydrophobic mismatch $u_0$ can be related to the membrane tension $\sigma$ via [7]

$$u_0 = \frac{U_0}{d_0} + \frac{\sigma}{K_a}, \quad (18)$$

where $U_0$ is the non-normalized excess thickness of the channel in the tensionless membrane. Following Ref. 7, the coefficients $C_0$ and $C_1$ of the channel lifetime are obtained from the Arrhenius law associated with the dimerization energy barrier:

$$-\frac{K_a d_0^2 F}{k_B T} = C_0 + C_1 \sigma + \mathcal{O}(\sigma^2), \quad (19)$$

where $k_B$ is Boltzmann's constant and $T$ the temperature. Note that the other (chemical) contributions to the dimerization energy do not depend on $\sigma$; therefore they will contribute to $C_0$ but not to $C_1$ [7].


[1] H. W. Huang, Biophys. J. **50**, 1061 (1986).

[2] T. Kim, K. I. Lee, P. Morris, R. W. Pastor, O. S. Andersen, and W. Im, Biophysical Journal **102**, 1551 (2012).

[3] I. Basu, A. Chattopadhyay, and C. Mukhopadhyay, Biochimica et Biophysica Acta (BBA) - Biomembranes **1838**, 328 (2014).

[4] L. Yang, T. A. Harroun, W. T. Heller, T. M. Weiss, and H. W. Huang, Biophysical journal **75**, 641 (1998).

[5] D. Constantin, Biochimica et Biophysica Acta (BBA) - Biomembranes **1788**, 1782 (2009).

[6] W. Rawicz, K. C. Olbrich, T. McIntosh, D. Needham, and E. Evans, Biophys J. **79**, 328 (2000).

[7] M. Goulian, O. N. Mesquita, D. K. Fygenson, C. Nielsen, O. S. Andersen, and A. Libchaber, Biophys. J. **74**, 328 (1998).

[8] P. Helfrich and E. Jakobsson, Biophys. J. **57**, 1075 (1990).

[9] A.-F. Bitbol, D. Constantin, and J.-B. Fournier, PLOS One **7**, e48306 (2012).

[10] S.-W. Chiu, S. Subramaniam, and E. Jakobsson, Biophysical Journal **76**, 1929 (1999).

[11] J. Yoo and Q. Cui, Biophysical Journal **104**, 117 (2013).

[12] A. H. Beaven, A. M. Maer, A. J. Sodt, H. Rui, R. W. Pastor, O. S. Andersen, and W. Im, Biophysical Journal **112**, 1185 (2017).
